# Supplementary material for: Routing and Wavelength Assignment with Protection: A Quadratic Unconstrained Binary Optimization Approach
Source: arXiv:2008.11924 source file (2021-06-08)
Supplement: Supplementary file 1 [file lemma_beta_models_equiv.tex]

\begin{lemma}
\label{lem:beta_models_equiv} [?????]
The models in \eqref{eq:prioritization_optmodel0} and \eqref{eq:prioritization_optmodel1} yield the same optimal values; that is, $\LBprioOne = \LBprioExact$. 
\end{lemma}

\proof{Proof.}
The feasible region of the model in \eqref{eq:prioritization_optmodel0} contains that of \eqref{eq:prioritization_optmodel1}, and hence $\LBprioOne \geq \LBprioExact$.
Moreover, since the condition in \eqref{eq:prioritization_optmodel1} implies \eqref{eq:prioritization_optmodel0} by Proposition \ref{prop:beta_model_onediff}, we have that $\LBprioOne \leq \LBprioExact$, which establishes that they are equal. \Halmos
